# Supplementary material for: Injecting Domain Adaptation with Learning-to-hash for Effective and Efficient Zero-shot Dense Retrieval
Source: arXiv:2205.11498 source file (2023-07-19)
Supplement: Supplementary file 1 [file bpr-backbone.tex]

\begin{table}[t]
    \small
    \centering
     \resizebox{0.45\textwidth}{!}{\begin{tabular}{l | c | c}
        \toprule
        \multicolumn{1}{c}{} & \multicolumn{2}{c}{\textbf{MSMARCO DEV}} \\ \midrule
        \multicolumn{1}{l|}{\textbf{BPR Models ($\downarrow$)}} & NDCG@10 & MRR@10 \\ \midrule
        \multicolumn{3}{c}{\textit{Fine-tuned models on MSMARCO}} \\ \midrule
        TAS-B & \textbf{0.397} & \textbf{0.336} \\
        MSMARCO-v3 (Dot) & 0.384 & 0.326 \\
        MSMARCO-v3 (Cosine) & 0.383 & 0.328 \\
        MiniLM-L6 & 0.362 & 0.306 \\ \midrule
        \multicolumn{3}{c}{\textit{Trained from Scratch}} \\ \midrule
        MSMARCO-v3 (Dot) & 0.368 & 0.312 \\
        MSMARCO-v3 (Cosine) & 0.375 & 0.320 \\ \midrule
        \multicolumn{3}{c}{\textit{Fine-tuned model on NQ}} \\ \midrule
        NQ \cite{yamada2021efficient} & 0.130 & 0.105 \\
    \bottomrule
    \end{tabular}}
    \caption{Backbone model analysis for BPR \cite{yamada2021efficient}. We evaluated both fine-tuned on MSMARCO or NQ or trained from scratch as backbones. TAS-B overall achieves the best in-domain BPR performances on the MSMARCO DEV dataset.}
    \label{tab:backbone-model-analysis}
\end{table}
